# Supplementary material for: Tracking the distance to criticality in systems with unknown noise
Source: arXiv:2310.14791 source file (2024-04-15)
Supplement: Supplementary file 2 [file arxiv_supp.tex]

% This file is used to include the contents of an .aux file in an arxiv submission. It should be updated manually with the contents of the relevant .aux file before zipping for arxiv. Past the contents of the file into the filecontents environment
